# Supplementary material for: Safe Reinforcement Learning via Shielding under Partial Observability
Source: arXiv:2204.00755 source file (2022-08-23)
Supplement: Supplementary file 1 [file noshield_ddqn_belief_supp.tex]

\addplot[dashed,red] table {%

};
