# Supplementary material for: Safe Reinforcement Learning via Shielding under Partial Observability
Source: arXiv:2204.00755 source file (2022-08-23)
Supplement: Supplementary file 2 [file noshield_dqn_belief_supp.tex]

\addplot[dashed,red] table {%
0.000000000000000000e+00 -1.008000000000000000e+03
1.000000000000000000e+03 -2.376000061035156250e+02
2.000000000000000000e+03 -2.603999938964843750e+02
3.000000000000000000e+03 -2.600000000000000000e+02
4.000000000000000000e+03 -2.607999877929687500e+02
5.000000000000000000e+03 -2.602000122070312500e+02
6.000000000000000000e+03 -2.603999938964843750e+02
7.000000000000000000e+03 -2.602000122070312500e+02
8.000000000000000000e+03 -2.597999877929687500e+02
9.000000000000000000e+03 -1.010200012207031250e+03
1.000000000000000000e+04 -2.593999938964843750e+02
};
