# Supplementary material for: Safe Reinforcement Learning via Shielding under Partial Observability
Source: arXiv:2204.00755 source file (2022-08-23)
Supplement: Supplementary file 7 [file shield_dqn_belief_supp.tex]

\addplot[red] table {%
0.000000000000000000e+00 -2.603999938964843750e+02
1.000000000000000000e+03 8.175000000000000000e+02
2.000000000000000000e+03 9.624000244140625000e+02
3.000000000000000000e+03 -2.366000061035156250e+02
4.000000000000000000e+03 8.537999877929687500e+02
5.000000000000000000e+03 9.559000244140625000e+02
6.000000000000000000e+03 9.667999877929687500e+02
7.000000000000000000e+03 -2.360000000000000000e+02
8.000000000000000000e+03 8.394000244140625000e+02
9.000000000000000000e+03 9.525999755859375000e+02
1.000000000000000000e+04 9.662000122070312500e+02
};
